# Supplementary material for: A physics-informed, vision-based method to reconstruct all deformation modes in slender bodies
Source: arXiv:2109.08372 source file (2021-09-17)
Supplement: Supplementary file 1 [file 04_Appendix.tex]

%\clearpage
%\appendix
